# Supplementary material for: Aharonov-Bohm interferences in polycrystalline graphene
Source: arXiv:1908.09399 source file (2019-08-25)
Supplement: Supplementary file 1 [file Nguyen_suppl.pdf]

# Supplementary Information for
# "Aharonov-Bohm interferences in polycrystalline graphene"

**V. Hung Nguyen and J.-C. Charlier**

*Institute of Condensed Matter and Nanosciences, Université catholique de Louvain,*
*Chemin des étoiles 8, B-1348 Louvain-la-Neuve, Belgium*

**Contents:**

***Sec. 1 - Magneto-transport through a single defect line in graphene.***
***Sec. 2 - Graphene grains and their boundaries investigated in Fig. 2 of the main text.***
***Sec. 3 - Effect of disorders at the grain boundary.***
***Sec. 4 - Magneto-transport in graphene systems with oxygen impurity barriers.***

## 1. Magneto-transport in graphene systems with a single defect line

Here, in order to demonstrate the skipping trajectories around the grain boundaries presented in Fig.1.c of the main text, we investigate magneto-transport in a simple case, i.e., across a single defect line (see the image on the top of Fig. 4 of the main text) in graphene systems. Here, we consider the perfectly ordered defect lines, which are experimentally achieved as in refs. [1,2].

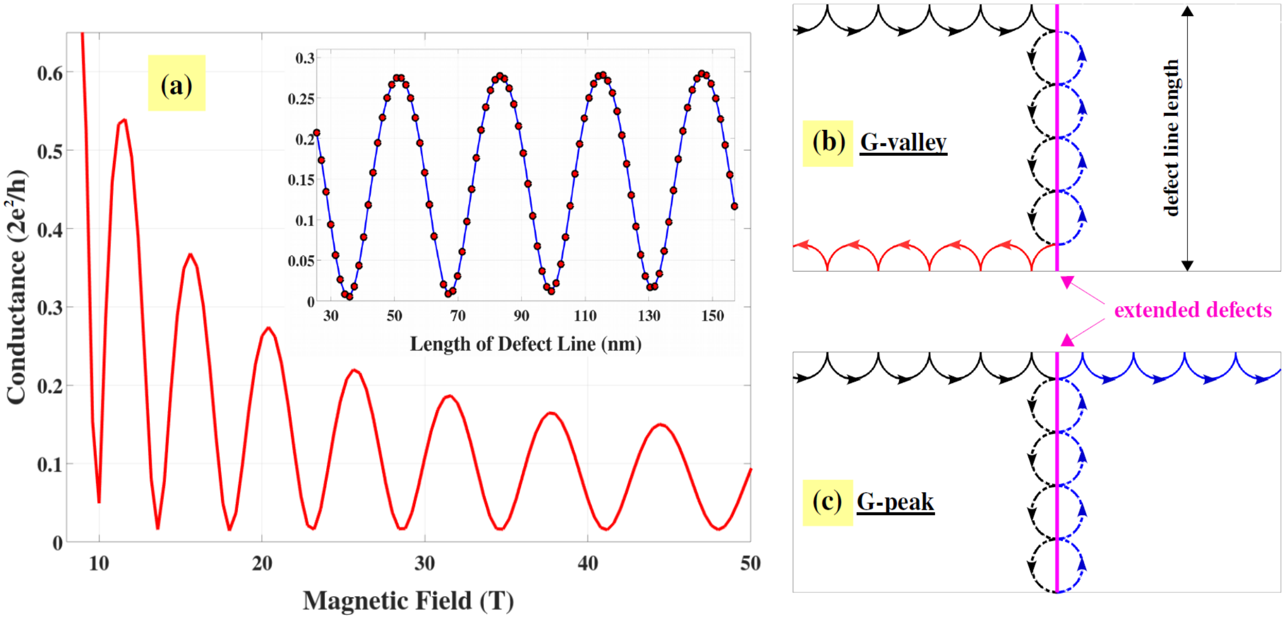


**Fig. S1**: *(a) Conductance as a function of magnetic field in a single defect line graphene system (see its atomic structure in Fig. 4 of the main text). The length (i.e., channel width, see in (b)) 80 nm of defect line and Fermi energy $E_F$ = 80 meV are considered. The inset of (a) displays the conductance at B = 20 T as a function of defect line length. (b,c) are simplified images to explain the observation of the conductance valley and peak, respectively.*

As discussed in the main text and presented in refs. [3-5], the electron propagation around the extended defects exhibits an essential difference (i.e., with opposite propagation directions in its two sides), compared to that obtained in graphene *p-n* junctions and *B*-field heterostructures (i.e., with a unique propagation direction). However, in both cases, electrons have to similarly follow cyclotron orbits when transmitting along the grain boundary / junction interface and hence one can anticipate that similar magneto-resistance oscillation, as those induced by snake trajectories in graphene *p-n* junctions and *B*-field heterostructures [6,7], can also be achieved in graphene systems with a single extended defect line. Indeed, such prediction is clearly confirmed by the results obtained and presented in Fig.S1.a. Similar to the effect of snake trajectories [7], simplified pictures of electron propagation to explain the conductance valley and peak in Fig. S1.a are diagrammatically presented in Fig.S1.b-c, respectively. Basically, the conductance should be determined by how the cyclotron radius compares to the length of defect line, therefore, is an oscillating function of both magnetic field and defect line length, as indeed seen in both Fig.S1.a and its inset.

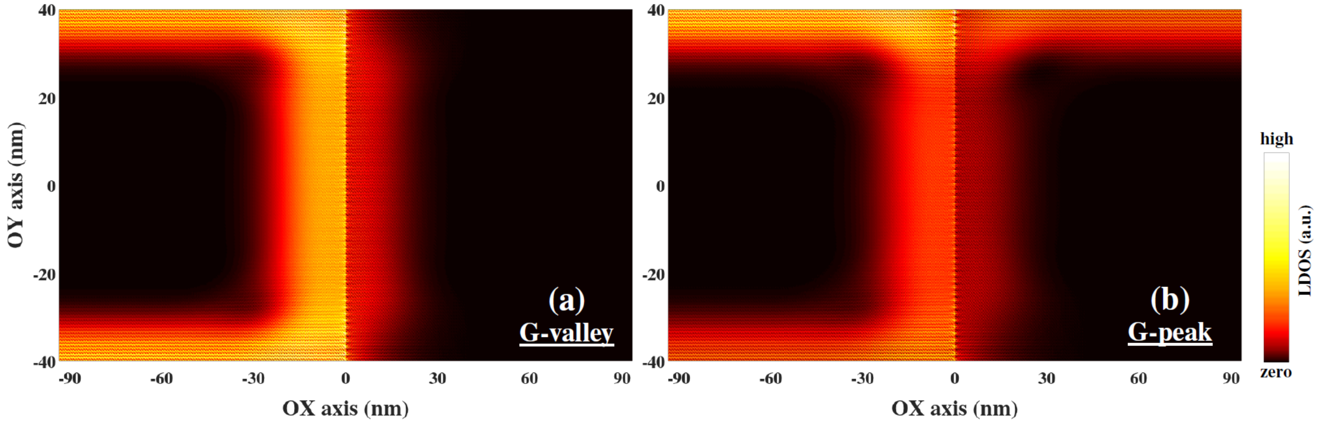


**Fig. S2**: *Local density of left-injected electronic states obtained at the conductance valley (B = 13.6 T in (a)) and peak (B = 11.6 T in (b)) in Fig.S1.*

Another clear evidence of the diagrammatical pictures in Figs. S1.b-c can be found in Fig.S2 where the local density of left-injected states reflecting the left-to-right propagation of electron wave computed at the conductance valley and peak, respectively, is displayed. Even though there is still a quantitative discrepancy between Fig.S1.c and the map in Fig. S2.b (i.e., backscatterings still occur), the qualitative consistency between the simplified diagrams in Figs. S1.b-c and the computed results in Fig.S2 explains essentially the magneto-conductance oscillations in Fig. S1.a, i.e., as mentioned above, the conductance should be essentially determined by the relationship between the cyclotron radius and the defect line length.

Thus, the investigation in this section clearly demonstrates the pictures of skipping trajectories presented and discussed in the main text.

## 2. Graphene grains and grain boundaries investigated in Fig. 2 of the main text

Fig.S3 presents a zoom of the atomic structure of the system investigated in Fig.2 of the main text. Even though the grains 1 and 3 are formed by the same graphene lattice (for simplicity), it represents three main structural properties, which can be practically obtained as in refs. [8,9], including irregular edges as illustrated in Fig.1.a of the main text, misorietation between the graphene grains (particularly,

a misorientation angle of 30° between grain 2 and grains 1 and 3) and structural disorders at the grain boundaries. Note that this grain boundary system corresponds to the (5,0)|(3,3) structure in ref. [10] that has been experimentally achieved in ref. [11]. In many works (e.g., refs. [10,12,13]) on this structure in the 2D form (i.e., infinite along the grain boundary axis), the grain boundary is assumed to be ordered with a short periodic length $d \approx 1.25$ nm, leading to a lattice mismatch of about 3.8% between these graphene grains. This lattice mismatch has been always solved by applying strains on either one of or both of them. In this work, we however considered a system where the grain boundary is large but finite (~ 55 nm) and contains structural disorders (see Fig.S3). The mentioned lattice mismatch is hence avoided. Note additionally that while the finite size of the internal grain (grain 2) (with a maximum width ~ 60 nm and a maximum length ~ 62 nm as investigated in the main text) is taken into account, the grains 1 and 3 are assumed to be large enough (particularly, long enough along the transport direction) so that they can act as semi-infinite left and right leads, respectively.

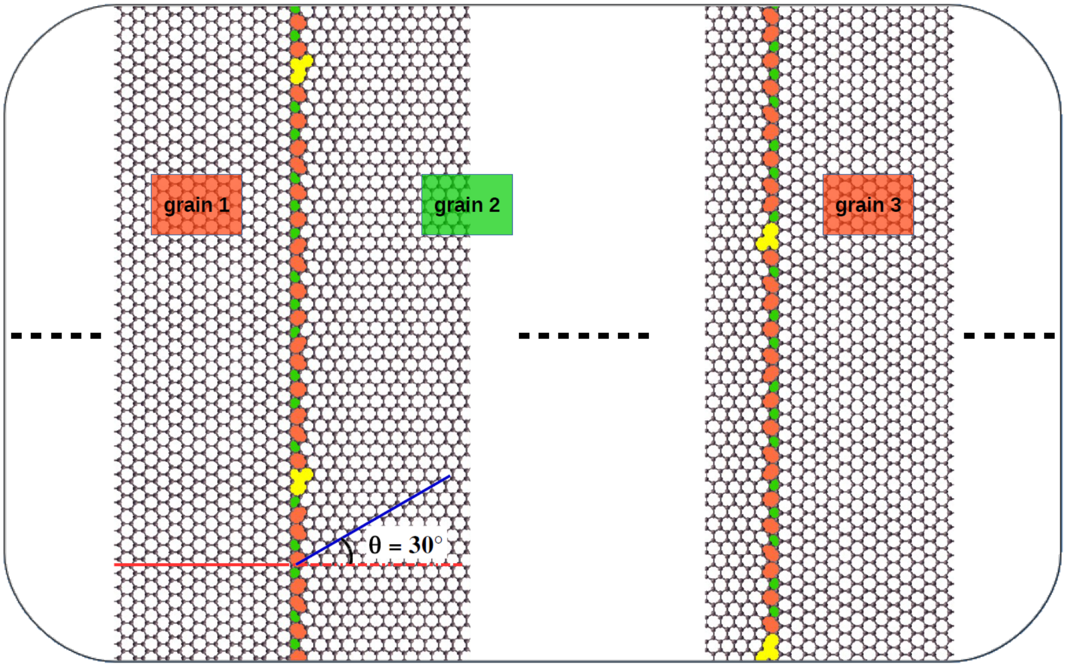


**Fig. S3**: *A zoom of the atomic structure of graphene grains and their boundaries investigated in Fig.2 of the main text.*

### 3. Effect of disorders at the grain boundary

In Fig.S4, the conductance as a function of magnetic field obtained in fifteen graphene systems containing different disordered defect lines is displayed. These disordered defect lines are modeled by introducing randomly vacancies around the ordered one as illustrated in Fig.4.a of the main text.

The obtained results show that even though the conductance is sensitive to the disorder effects, strong Aharonov-Bohm oscillations can still be observed in all these considered cases, thus demonstrating that this interference is quite robust under the effect of these disorders.

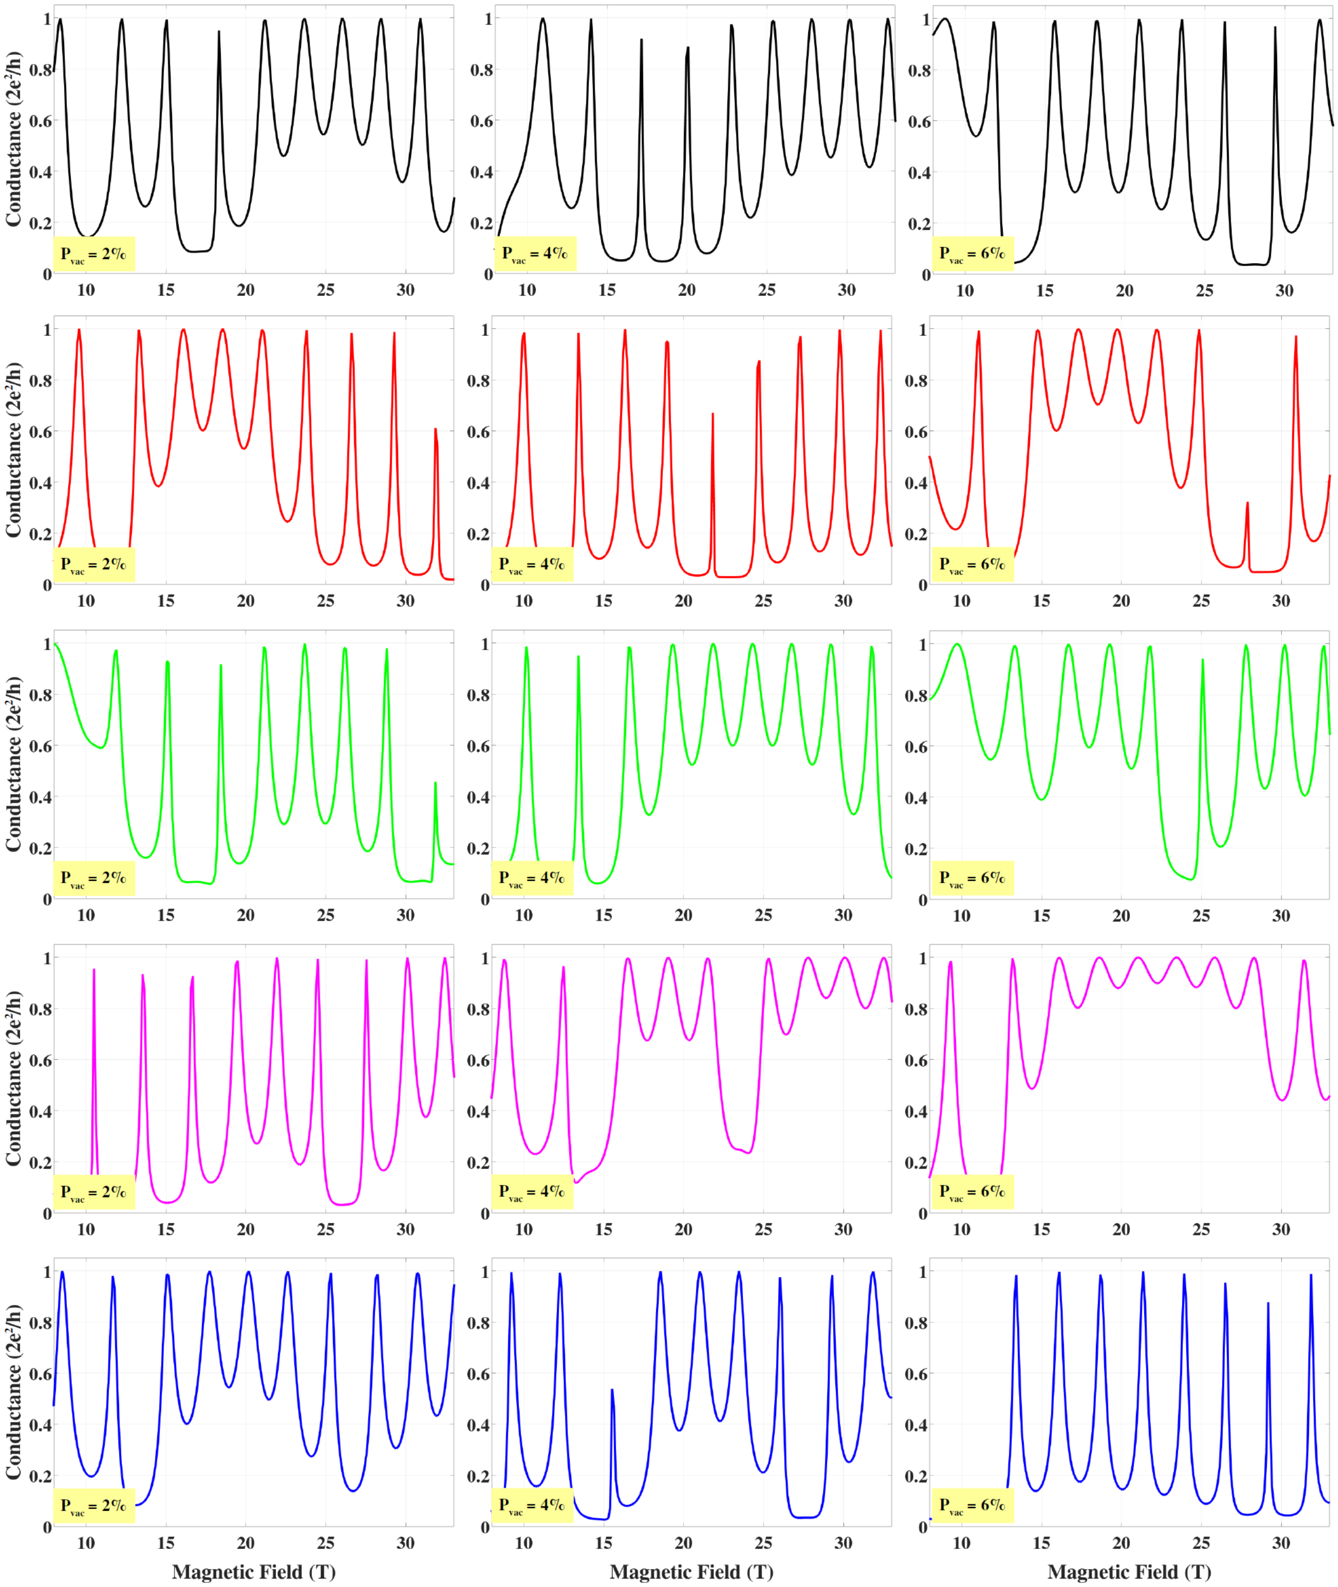


**Fig. S4**: *Aharonov-Bohm interferences in graphene nanoribbon with different disordered defect lines. In particular, we investigate the systems, similar to those in Fig.4 of the main text, where vacancies are randomly introduced around the ordered defect line with different probabilities:* $P_{vac}$ *= 2% (left), 4%(middle) and 6% (right panels).*

### 4. Magneto-transport in graphene systems with oxygen impurity barriers

In this section, we would like to explain in more detail our calculations for graphene systems with oxygen impurity barriers.

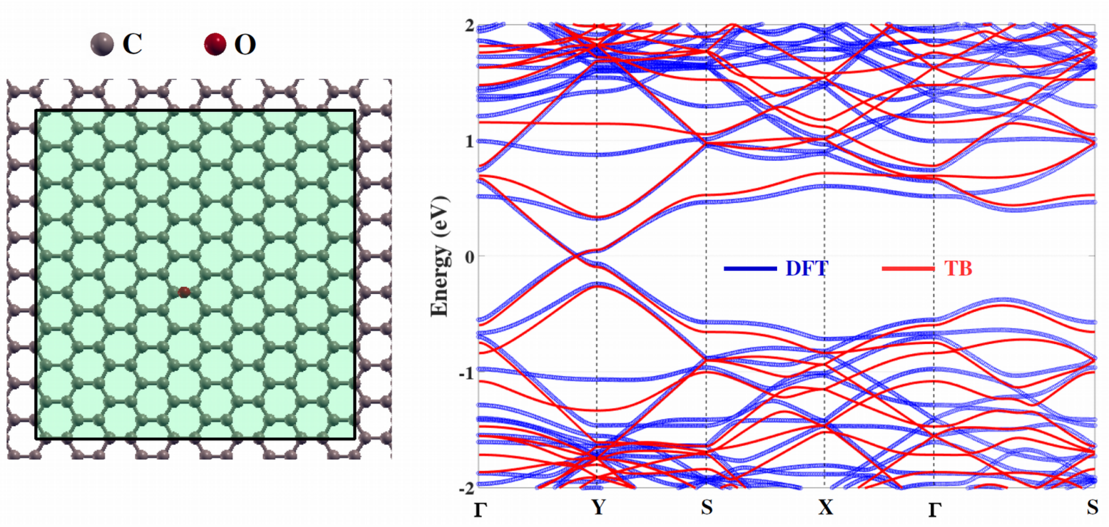


**Fig. S5**: *Tight binding vs DFT calculations for graphene with oxygen impurities: top view of the periodic unit cell used in calculations (left) and obtained electronic bandstructures (right).*

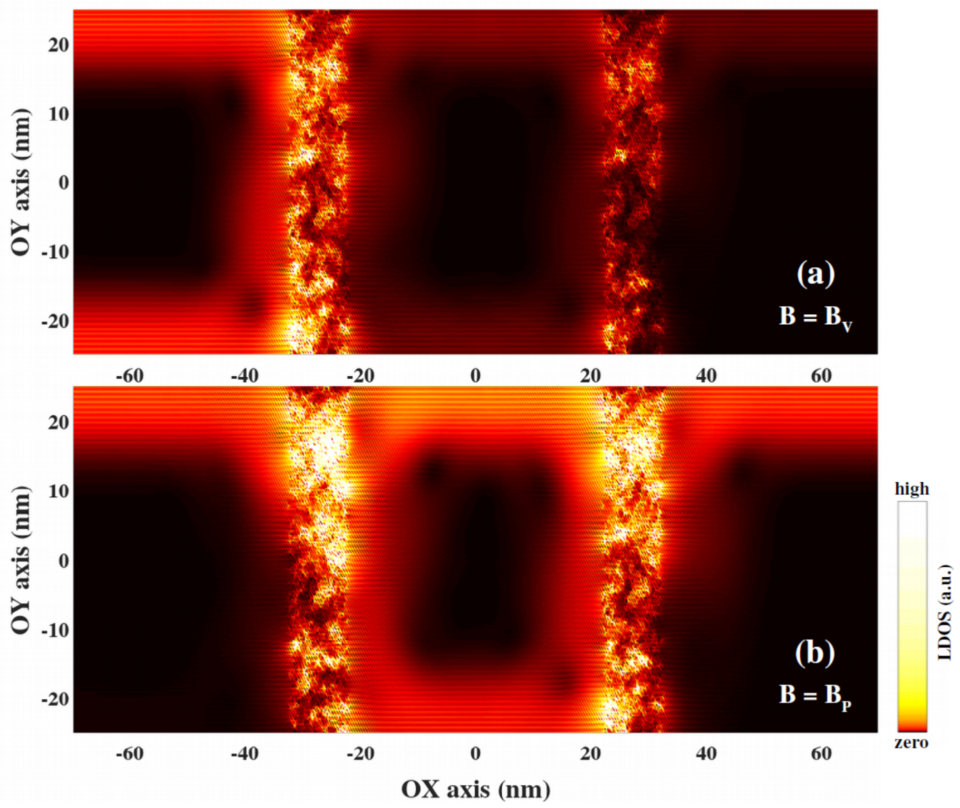


**Fig. S6**: *Local density of left-injected electronic states obtained at the conductance valley (a) and peak (b) at the V- and P-points in the top-left panel of Fig.S7, respectively, of a graphene system with two oxygen impurity barriers.*

First, to compute the electronic properties of graphene with oxygen impurities, we performed Density Functional Theory (DFT) calculations [14]. The simple $p_z$ tight-binding Hamiltonian is then adjusted to fit with the obtained DFT data. Some adjusted tight-binding models have been actually investigated [15,16] to model the effects of oxygen impurities in graphene. However, focusing only on the transport of low energy carriers, we further considered these models and propose a simpler one based on the nearest neighbor Hamiltonian that has been widely used in the literature (also in this work) to model pristine graphene. As explained in the main text, the effects of impurities are effectively modeled by adding an on-site energy $\varepsilon_{on}$ = 28 eV to carbon sites directly interacting with the impurity. The validity of this model is demonstrated in Fig.S5 as it reproduces quite accurately the low energy ($|E| \lesssim 0.5$ eV) DFT bandstructure of the considered graphene system.

This simply adjusted model was then employed to compute the magneto-transport through graphene systems with two oxygen impurity barriers in this work.

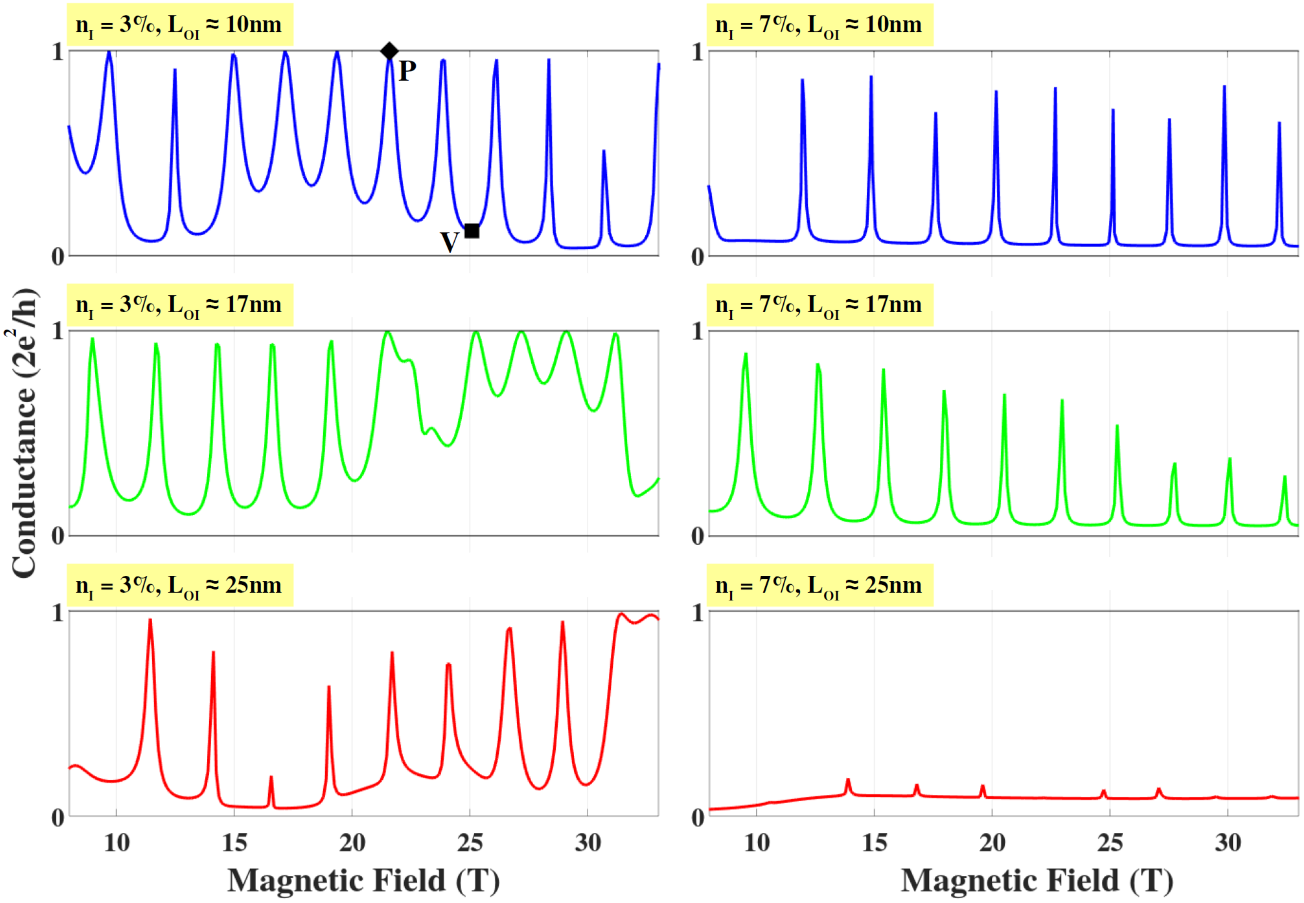


**Fig. S7**: *Aharonov-Bohm interferences in graphene nanoribbons with two oxygen impurity barriers. The impurity density is* $n_I$ *= 3% and 7% for the left and right panels, respectively. The barrier width is* $L_{OI}$ *≈ 10 nm (for top), ≈ 17 nm (middle) and ≈ 25 nm (bottom panels).*

Fig. S6 presents typical pictures of electron propagation through these oxygen impurity barrier systems at the destructive (see Fig.S6.a, corresponding to a conductance valley) and constructive (see Fig.S6.b, corresponding to a conductance peak) states, indeed showing the similarity, as discussed in the main text, between the effects of functional impurities and structural defects when using to design Aharonov-Bohm interferometers.

The results obtained when increasing the width of oxygen impurity barriers are displayed in Fig.S7. Basically, similar to the effects of impurity density discussed in the main text, the observed Aharonov-Bohm effect is degraded when increasing the width of impurity barriers and additionally the degradation rate is larger for a larger impurity density.

**References:**


[1] J. Lahiri, Y. Lin, P. Bozkurt, I. I. Oleynik, M, Batzill, Nat. Nanotechnol. **5**, 326-329 (2010).
[2] J.-H. Chen et al., Phys. Rev. B **89**, 121407(R) (2014).
[3] A. W. Cummings, A. Cresti, and S. Roche, Phys. Rev. B **90**, 161401(R) (2014).
[4] A. Bergvall, J. M. Carlsson, and T. Lfwander, Phys. Rev. B **91**, 245425 (2015).
[5] M. Phillips and E. J. Mele, Phys. Rev. B **96**, 041403(R) (2017).
[6] P. Rickhaus, P. Makk, M.-H. Liu, E. Tóvári, M. Weiss, R. Maurand, K. Richter, and C. Schönenberger, Nat. Commun. **6**, 6470 (2015).
[7] L. Oroszlány, P. Rakyta, A. Kormányos, C. J. Lambert, and J. Cserti, Phys. Rev. B **77**, 081403(R) (2008).
[8] Q. Yu *et al.*, Nat. Mater. **10**, 443-449 (2011).
[9] P. Yasaei *et al.*, Nat. Commun. **5**, 4911 (2014).
[10] O. V. Yazyev and S. G. Louie, Nat. Mater. **9**, 806-809 (2010).
[11] H. I. Rasool, C. Ophus, W. S. Klug, A. Zettl, and J. K. Gimzewski, Nat. Commun. **4**, 2811 (2013).
[12] S. B. Kumar and J. Guo, Nano Lett. **12**, 1362-1366 (2012).
[13] V. Hung Nguyen, T. X. Hoang, P. Dollfus and J.-C. Charlier, Nanoscale **8**, 11658-11673 (2016).
[14] http://www.openmx-square.org
[15] N. Leconte *et al.*, ACS Nano **4**, 4033-4038 (2010).
[16] N. Leconte *et al.*, Phys. Rev. B **84**, 235420 (2011).
